# Supplementary material for: Electronic Properties of Defective MoS$_{2}$ Monolayers Subject to Mechanical Deformations: A First-Principles Approach
Source: arXiv:1904.12706 ancillary file (2019-12-12)
Supplement: Supplementary file 1 [file supplementaryinfo.pdf]

# Supplementary Information for "Electronic Properties of Defective $MoS_2$ Monolayers Subject to Mechanical Deformations: A First-Principles Approach"

**Mohammad Bahmani[*,1], Mahdi Faghihnasiri[2], Michael Lorke[1], Agnieszka-Beata Kuc[3,4] Thomas Frauenheim[1]**

[1] Bremen Center for Computational Materials Science, Department of Physics, Bremen University, Am Fallturm 1, 28359 Bremen, Germany
[2] Computational Materials Science Laboratory, Nano Research and Training Center, 1478934371 Tehran, Iran
[3] Helmholtz-Zentrum Dresden-Rossendorf, Department of Resource Ecology, Research Center Leipzig, Permoser 15, 04318 Leipzig, Germany
[4] Department of Physics & Earth Science, Jacobs University Bremen, 28759 Bremen, Germany

**Key words:** $MoS_2$, electronic structure, defects, strain engineering, two-dimensional materials

* Corresponding author: e-mail mbahmani@uni-bremen.de

**Monolayers (ML) of Group-6 transition-metal dichalcogenides (TMDs) are semiconducting two-dimensional materials with direct bandgap, showing promising applications in various fields of science and technology, such as nanoelectronics and optoelectronics. These monolayers can undergo strong elastic deformations, up to about 10%, without any bond breaking. Moreover, the electronic structure and transport properties, which define the performance of these TMDs monolayers in nanoelectronic devices, can be strongly affected by the presence of point defects, which are often present in the synthetic samples. Thus, it is important to understand both effects on the electronic properties of such monolayers. In this work, we have investigated the electronic structure and energetic properties of defective $MoS_2$ monolayers, as subject to various strains, using density functional theory simulations. Our results indicated that strain leads to strong modifications of the defect levels inside the bandgap and their orbital characteristics. Strain also splits the degenerate defect levels up to an amount of 450 meV, proposing novel applications.**

Copyright line will be provided by the publisher

Copyright line will be provided by the publisher

## Supplementary Information

**This file includes:**

1. Displacement map of the ML $MoS_2$ with defects to highlight the importance of the geometry optimization in studying their properties.
2. Results and discussions for $V_S$ under four types of strain.
3. The orbital characteristics of localized DLs as a function of various applied strains for $V_S$, $V_{2S-top}$, $V_{2S-top}$, and $V_{Mo}$.
4. The change in the geometry of the atoms surrounding the $V_{Mo}$ inside ML $MoS_2$.
5. The shift in the defect levels as well as the band edges for ML $MoS_2$ with $V_{Mo+3S}$ and $V_{Mo+6S}$ complex vacancies.
6. The input parameters for the self-generated pseudopotentials.

**Displacement map of surrounding atoms**In Fig. S1, we show the displacement, in Å, of atoms in the ML $MoS_2$ surrounding defects compare to their position in the pristine structure. $V_{Mo}$ has very small impact on the neighboring atoms. As it is shown in these figures, atomic positions are mostly renormalized by the presence of $V_{2sv-par}$, and $V_{Mo+6S}$ in monolayers. For the case of $V_S$ and $V_{Mo+3S}$ vacancies the neighbors are moved more than $V_{2S-top}$.

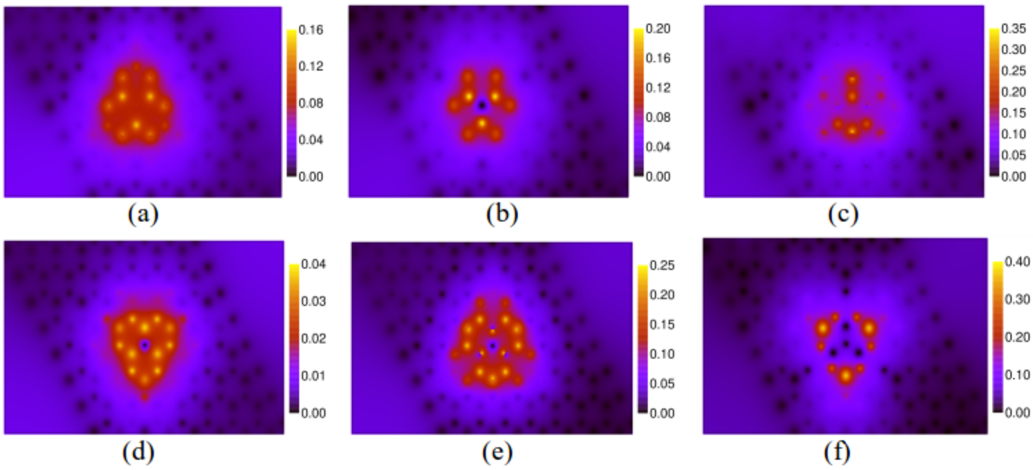


**Figure 1** (Color online) The displacement map of atoms in the $MoS_2$ ML surrounding defects as a) $V_S$, b) $V_{2S-top}$, c) $V_{2sv-par}$, d) $V_{Mo}$, e) $V_{Mo+3S}$, f) $V_{Mo+6S}$. All the numbers in the colorboxes are in Å.

**$V_S$ vacancy** In Figs. S2(a)–(d), studying the ML $MoS_2$ with $V_S$, we display the evolution of the band edges and DLs of a sulfur vacancy, $V_S$, under four types of strain. The black lines are band edges and the green dashed-line displays the Fermi level's position. The colored lines indicate the states DL1, DL2, and DL3. Here, we are only interested in the double-degenerate empty states close to the Fermi level. In the unstrained monolayer, DL2 and DL3 are mostly composed of $d_{xy}$ and $d_{x^2-y^2}$ orbitals of the neighboring molybdenums, respectively, as shown in Fig. S3. Their degeneracy is lifted under uniaxial and shear T1 strains since the hexagonal symmetry is removed. Besides, isotropic biaxial strain does not split the degenerate levels and just move them closer to the CBM. The uniaxial strain in X-direction tunes DL2 more than

Copyright line will be provided by the publisher

DL3, but strain in Y-direction shifts DL3 more than DL2. In addition, shear T1 strain makes a mixture of contributions $d_{xy}$ and $d_{x^2-y^2}$ orbitals to DL2 and DL3. As shown in Figs. S2(d),(e), shear T1 does not influence much the band edges though degeneracy splitting is noticeable. However, in all the cases, the position of the occupied shallow level stays almost unchanged. Fig. S2(e) illustrates the amount of degenerate levels' separation in the same interval of strain for four types of strains. Even a small quantity, around $\pm 2\%$, of uniaxial or shear T1 strain enhances the level separation to around 60 or 110 meV, respectively. Further increasing the tensile shear T1 strain splits the levels up to almost 260 meV at $+5\%$.

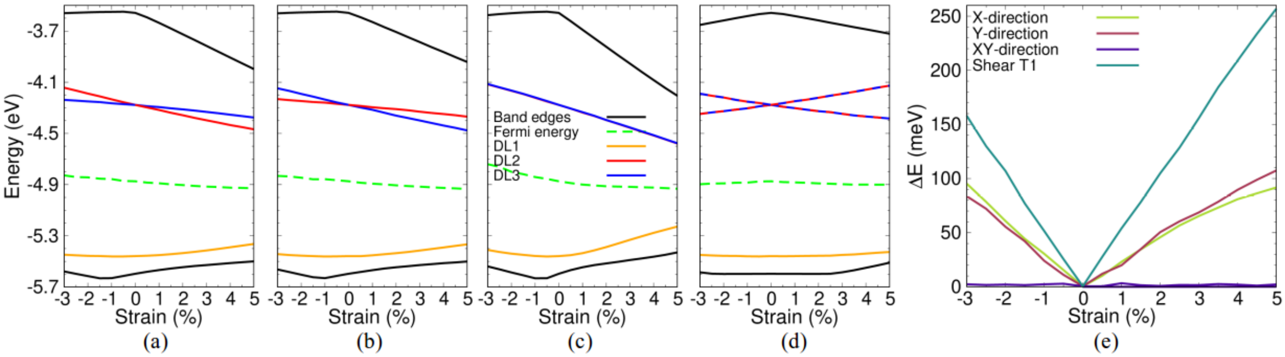


**Figure 2** (Color online) Evolution of the band edges along with the DLs of the $MoS_2$ ML with $V_S$ under strain in a) X-direction, b) Y-direction, c) XY-direction, and d) shear T1. The Fermi level and band edges are indicated with green dashed-line and black lines, respectively. The defect states, DL1–DL5, are shown with orange, red, blue, gray, and magenta line, respectively. e) The amount of degeneracy splitting of the deep DLs is plotted in the same interval for all four strains.

Fig. S3 displays the orbital characteristics of vacancy states for $V_S$ in ML $MoS_2$ as a function of strain along X-direction, Y-direction, and shear T1. In these images, blue and red orbitals, plotted at isosurface of 0.2 $\AA^{-3}$, corresponds to the lower and higher energy DLs at the zero strain, respectively. The orbitals' color of each band stay the same for all the strain cases except shear T1 which mixes the orbital components. Under uniaxial strain, the localized defect states are displayed with similar coloring. However, the defect levels are shown with cyan and magenta orbitals for compression and tensile shear T1 strains due to their orbital mixing.

**$V_{2S-top}$ vacancy** In Fig. S4, we show the orbital characteristics of deep DLs close to the Fermi energy for $V_{2S-top}$ in ML $MoS_2$ as a function of strain along X-direction, Y-direction, and shear T1 strain. In these images, blue and red orbitals, plotted at isosurface of 0.2 $\AA^{-3}$, corresponds to the lower and higher energy DLs at the zero strain, respectively. The orbitals' color of each band stay the same for all the strain cases except shear T1 which mixes the orbital components. Under uniaxial strain, the localized defect states are displayed with similar coloring. However, under compression and tensile shear T1 strains, the DLs are shown with cyan and magenta orbitals due to their orbital mixing.

**$V_{2S-par}$ vacancy** We display the orbital characteristics of $V_{2S-par}$ in ML $MoS_2$ for strain along X-direction, Y-direction, and shear T1 strain, as depicted in Fig. S5. In these images, blue and red orbitals, plotted at isosurface of 0.2 $\AA^{-3}$, corresponds to the lower and higher energy DLs at the zero strain, respectively. The orbitals' color of each band stay the same for all the strain cases except shear T1 which mixes the orbital components. Under uniaxial strain, the localized

Copyright line will be provided by the publisher

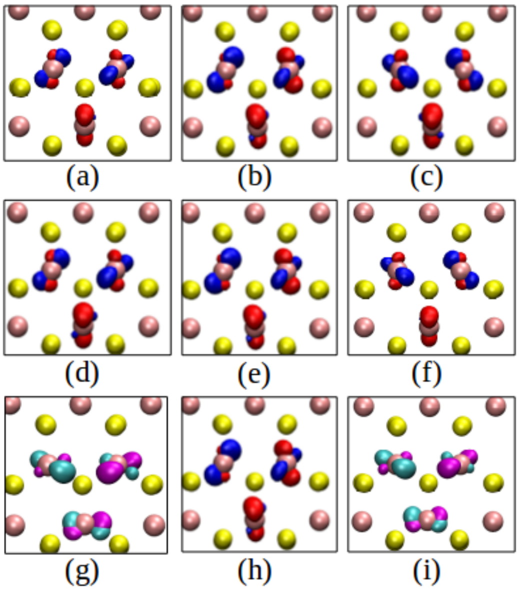


**Figure 3** (Color online) Orbital characteristics of unoccupied deep DLs of $V_S$ in ML $MoS_2$ at a) -3.0%, b) 0.0%, and c) +3.0% strain in X-direction, and d) -3.0%, e) 0.0%, and f) +3.0% strain in Y-direction, and g) -1.5%, h) 0.0%, and i) +1.0% shear T1 strain. The red and blue orbitals, plotted at isosurface of 0.2 $\mathring{A}^{-3}$, are indicating the DLs at zero strain, respectively, which also label the localized states of the monolayers under strain in X- and Y-direction. In the case of shear T1 strain, DLs are displayed with cyan and magenta orbitals due to their orbital mixing.

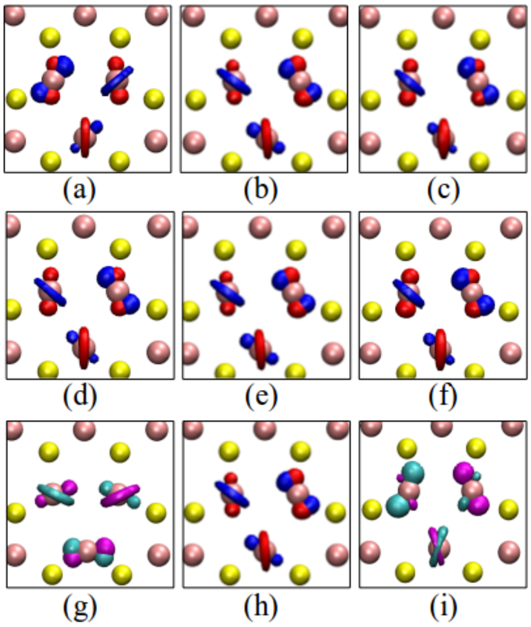


**Figure 4** (Color online) Orbital characteristics of unoccupied deep DLs of $V_{2S-top}$ in Ml $MoS_2$ at a) -3.0%, b) 0.0%, and c) +5.0% strain in X-direction, and d) -3.0%, e) 0.0%, and f) +3.0% strain in Y-direction, and g) -1.0%, h) 0.0%, and i) +1.0% shear T1 strain. The red and blue orbitals, plotted at isosurface of 0.2 $\mathring{A}^{-3}$, are indicating the DLs at zero strain, respectively, which also label the localized states of the monolayers under strain in X- and Y-direction. In the case of shear T1 strain, DLs are displayed with cyan and magenta orbitals.

defect states are displayed with similar coloring. However, under compression and tensile shear T1 strains, the DLs are shown with cyan and magenta orbitals due to their orbital mixing. strains.

Copyright line will be provided by the publisher

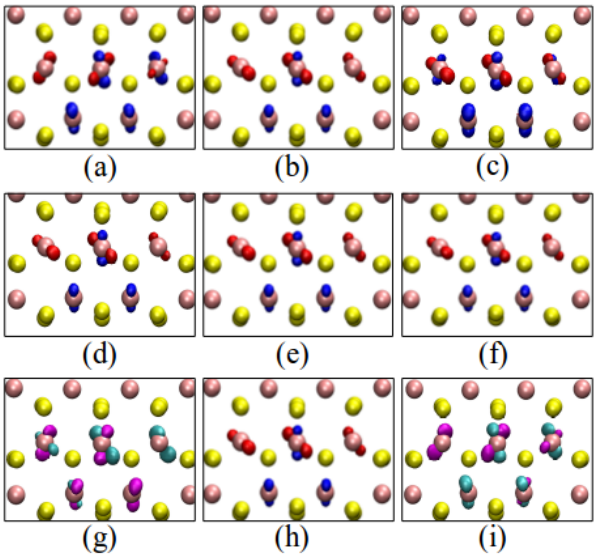


**Figure 5** (Color online) Orbital characteristics of unoccupied deep DLs of $V_{2S-par}$ in ML $MoS_2$ at a) +1.0%, b) 0.0%, and c) +3.0% strain in X-direction, and d) -1.5%, e) 0.0%, and f) +3.0% strain in Y-direction, and g) -1.0%, h) 0.0%, and i) +1.0% shear T1 strain. The red and blue orbitals, plotted at isosurface of 0.2 $\AA^{-3}$, are indicating the DLs at zero strain, respectively, which also label the localized states of the monolayers under strain in X- and Y-direction. In the case of shear T1 strain, DLs are displayed with cyan and magenta orbitals.

**$V_{Mo}$ vacancy** In Fig. S6, we illustrate the orbital characteristics of deep DLs close to the Fermi energy for ML $MoS_2$ with $V_{Mo}$ as a function of strain along X-direction, Y-direction, and shear T1 strain. The orbitals are plotted at isosurface of 0.2 $\AA^{-3}$ and colored based on their energies, from the lowest to the highest, their color is blue, red, gray, orange, cyan, and magenta, respectively. These strains change the CBM, below which introduce an empty shallow DL. This band is constituted of $d_{x^2-y^2}$ and $d_{xy}$ in case of compression in X-direction and $d_{x^2-y^2}$, $d_{xy}$, and a small portion of $p_x$ for compression and tensile in Y-direction.

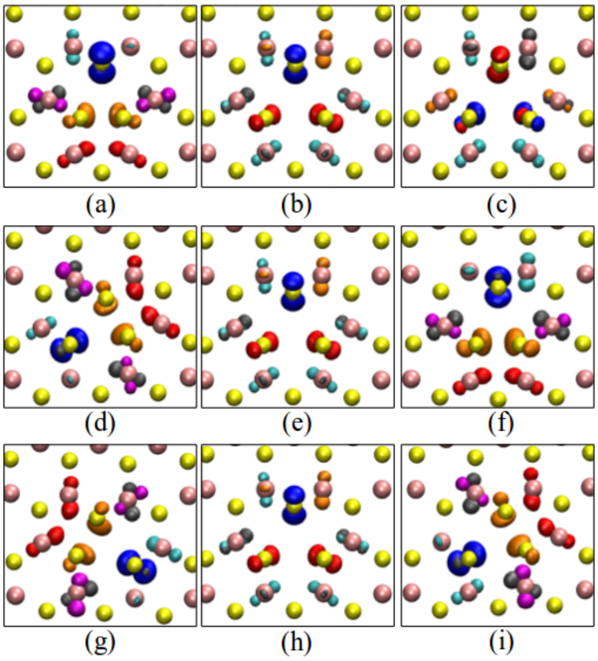


**Figure 6** (Color online) Orbital characteristics of unoccupied deep DLs of $V_{Mo}$ in ML $MoS_2$ at a) -1.0%, b) 0.0%, and c) +1.0% strain in X-direction, and d) -1.5%, e) 0.0%, and f) +2.0% strain in Y-direction, and g) -1.0%, h) 0.0%, and i) +1.0% shear T1 strain. The orbitals are plotted at isosurface of 0.2 $\AA^{-3}$ and colored based on their energies, from the lowest to the highest, their color is blue, red, gray, orange, cyan, and magenta, respectively.

Copyright line will be provided by the publisher

**Geometry modifications for ML $MoS_2$ with $V_{Mo}$** In Fig. S7, we show the change in the position of the neighboring atoms around a Mo vacancy inside ML $MoS_2$, under different strains. The dramatic modification of the monolayers is depicted which leads to the breaking of the "$C_{3v}$" symmetry.

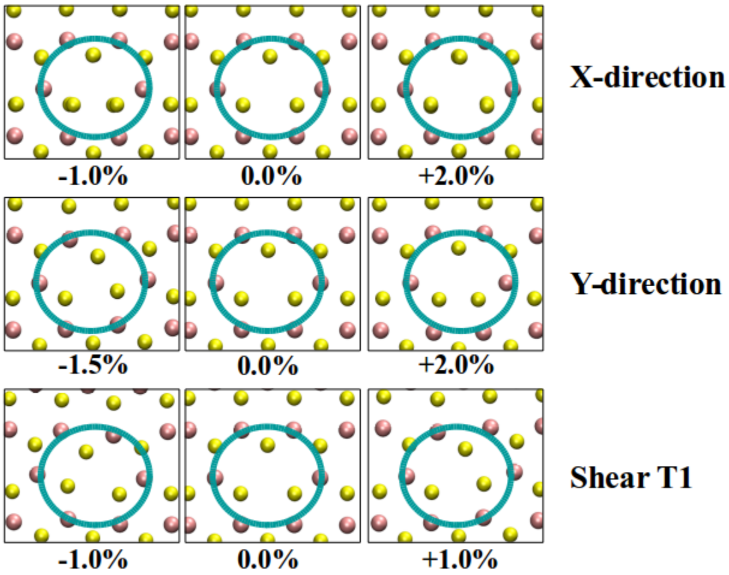


**Figure 7** (Color online) The change in the position of the atoms surrounding $V_{Mo}$ in ML $MoS_2$ at first row) -1.0%, 0.0%, +2.0% strain in X-direction, and second row) -1.5%, 0.0%, and +2.0% strain in Y-direction, and third row) -1.0%, 0.0%, and +1.0% shear T1 strain. The position of the vacancy and its neighboring sulfurs are highlighted with a cyan circle.

**$V_{Mo+3S}$ and $V_{Mo+6S}$ vacancies** The evolution of the band edges and localized DLs of $V_{Mo+3S}$ and $V_{Mo+6S}$ are demonstrated in Figs. S8 and S9, respectively. The black lines are band edges and the green dashed-line displays the Fermi levels position. The colored lines indicate the states DL1–DL8. As it can be seen, the change in geometry and hybridization of the orbital components result in the modification and mixing of the defect bands. However, it can still be observed that compressive and tensile uniaxial and biaxial strains shift the CBM but not the VBM. In both cases, shear T1 strain does not modify the band edges.

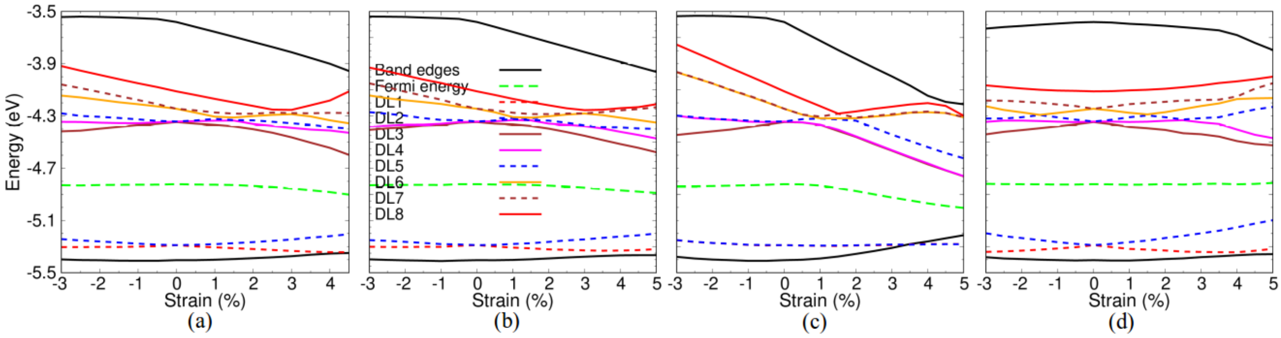


**Figure 8** (Color online) Evolution of the band edges along with the DLs of ML $MoS_2$ with $V_{Mo+3S}$ under strain in a) X-direction, b) Y-direction, c) XY-direction, and d) shear T1. In all the plots, Fermi level and band edges are indicated with green dashed-line and black lines, respectively. Other colored lines represent DLs.

Copyright line will be provided by the publisher

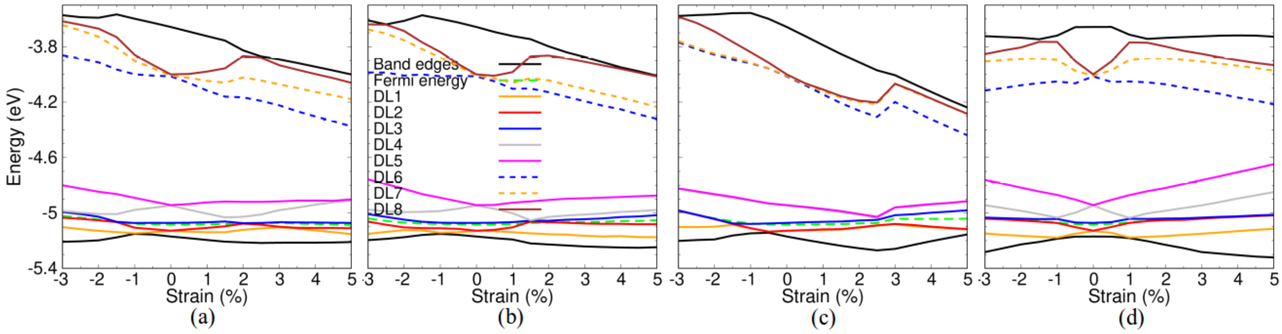


**Figure 9** (Color online) Evolution of the band edges along with the DLs of ML $MoS_2$ with $V_{Mo+6S}$ under strain in a) X-direction, b) Y-direction, c) XY-direction, and d) shear T1. In all the plots, Fermi level and band edges are indicated with green dashed-line and black lines, respectively. Other colored lines represent DLs.

**Input parameters for the self-generated pseudopotentials** The set of pseudopotentials used in these studies are self-generated by means of *"atom"* tool which is provided by SIESTA's developers along with the source code. The tool and an instruction of how to generate the pseudopotentials can be found under the *"/Util/Gen-basis/"* directory. Here are the input parameters which we used to produce:

**Pseudopotential for Mo:**

```
%define NEW_CC
   pe                -- file generated from Mo ps file
        tm2
   Mo   pbr
     0.000     0.000     0.000     0.000     0.000     0.000
    8    4
    5    0     1.000     0.000    #5s
    5    1     0.000     0.000    #5p
    4    2     5.000     0.000    #4d
    4    3     0.000     0.000    #4f
    2.50000   3.00000   1.40000   2.20000   0.00000   2.55000   Core corrs

#234567890123456789012345678901234567890123456789012345678901234567890      Ruler
```

**Pseudopotential for S:**

```
%define NEW_CC
   pe    Sulphur
        tm2     2.08
    S   pbr
       0.00     0.00     0.00     0.00     0.00     0.00
```

```
   3    4
   3    0       2.00       0.00
   3    1       4.00       0.00
   3    2       0.00       0.00
   4    3       0.00       0.00
  1.78      1.94      2.29      2.29      0.00     1.51

1234567890123456789012345678901234567890      Ruler
```

Copyright line will be provided by the publisher
